# Supplementary material for: Molecular beam homoepitaxy of N-polar AlN: enabling role of Al-assisted surface cleaning
Source: arXiv:2204.08604 source file (2022-04-19)
Supplement: Supplementary file 1 [file Supplemental.pdf]

# Supplementary Materials for

## Molecular beam homoepitaxy of N-polar AlN: enabling role of Al-assisted surface cleaning

Zexuan Zhang,[1] Yusuke Hayashi,[2] Tetsuya Tohei,[2] Akira Sakai,[2] Vladimir Protasenko,[1] Jashan Singhal,[1] Hideto Miyake,[3,4] Huili Grace Xing,[1,5,6] Debdeep Jena,[1,5,6] and YongJin Cho[1]

[1]*School of Electrical and Computer Engineering, Cornell University, Ithaca, New York 14853, USA*
[2]*Graduate School of Engineering Science, Osaka University, 1-3 Machikaneyama-cho, Toyonaka, Osaka 560-8531, Japan*
[3]*Graduate School of Engineering, Mie University, 1577 Kurimamachiya-cho, Tsu, Mie 514-8507, Japan*
[4]*Graduate School of Regional Innovation Studies, Mie University, 1577 Kurimamachiya-cho, Tsu, Mie 514-8507, Japan*
[5]*Department of Materials Science and Engineering, Cornell University, Ithaca, New York 14853, USA*
[6]*Kavli Institute for Nanoscale Science, Cornell University, Ithaca, New York 14853, USA*

*Corresponding author. Email: zz523@cornell.edu and yongjin.cho@cornell.edu

**This PDF file includes:**

Supplementary Text
Figs. S1 to S2
References (*30*)

**Supplementary Text**

Microstructures of the defects in AlN samples were studied using cross-sectional (S)TEM. The actual nature of the defects was identified using cross-sectional TEM (Fig. S2), where the Burgers vector b of threading dislocations are determined by adjusting the diffraction vector g using the g·b=0 criterion. Non centrosymmetric reflection g=0002 and 000-2 were also used to detect any inversion domains which appear as contrast inversion in images taken with these diffraction vectors (*30*).

AlN directly grown on AlN template, the surface of which was not in situ cleaned (sample A), reveals a high density of structural defects that nucleate at the growth interface (Fig. S1A). Most of the defects in this AlN was identified to be a-type threading dislocations. It is interesting to note that despite the very high level of structural disorder at the AlN nucleation (Fig. 2B) the film reveals a single polarity, as evidenced by no image contrasts in Figs. S2 (B and C).

In contrast, AlN film grown on AlN template prepared by Al-assisted surface cleaning (sample B) shows only threading dislocations originating from the AlN template without any defects nucleated at the growth interface like sample A (Fig. S1B). These threading dislocations are characterized as a-type and the MBE-grown AlN layer displays a single N polarity (Figs. 6 and S2, D to F).

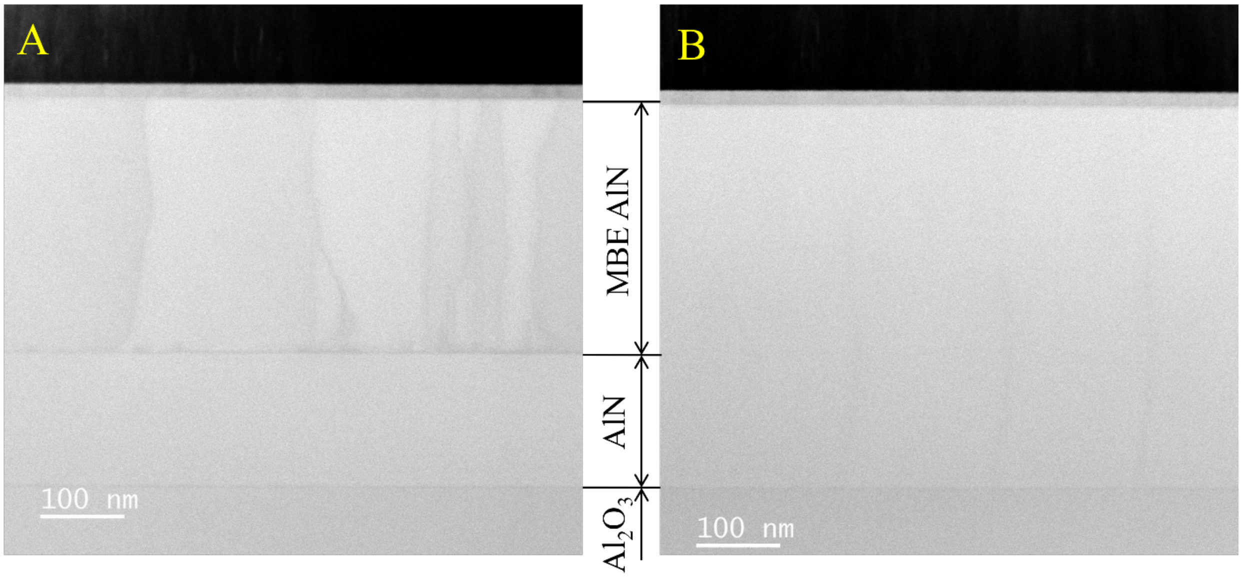


**Fig. S1.**

**Bright-field STEM images of AlN grown on AlN templates. (A)** Sample A, the substrate of which was not *in-situ* cleaned and **(B)** sample B, the substrate of which was Al-assisted cleaned. Note the defective interface structure and dislocations formed at the interface of sample A in (**A**), which are absent in sample B.

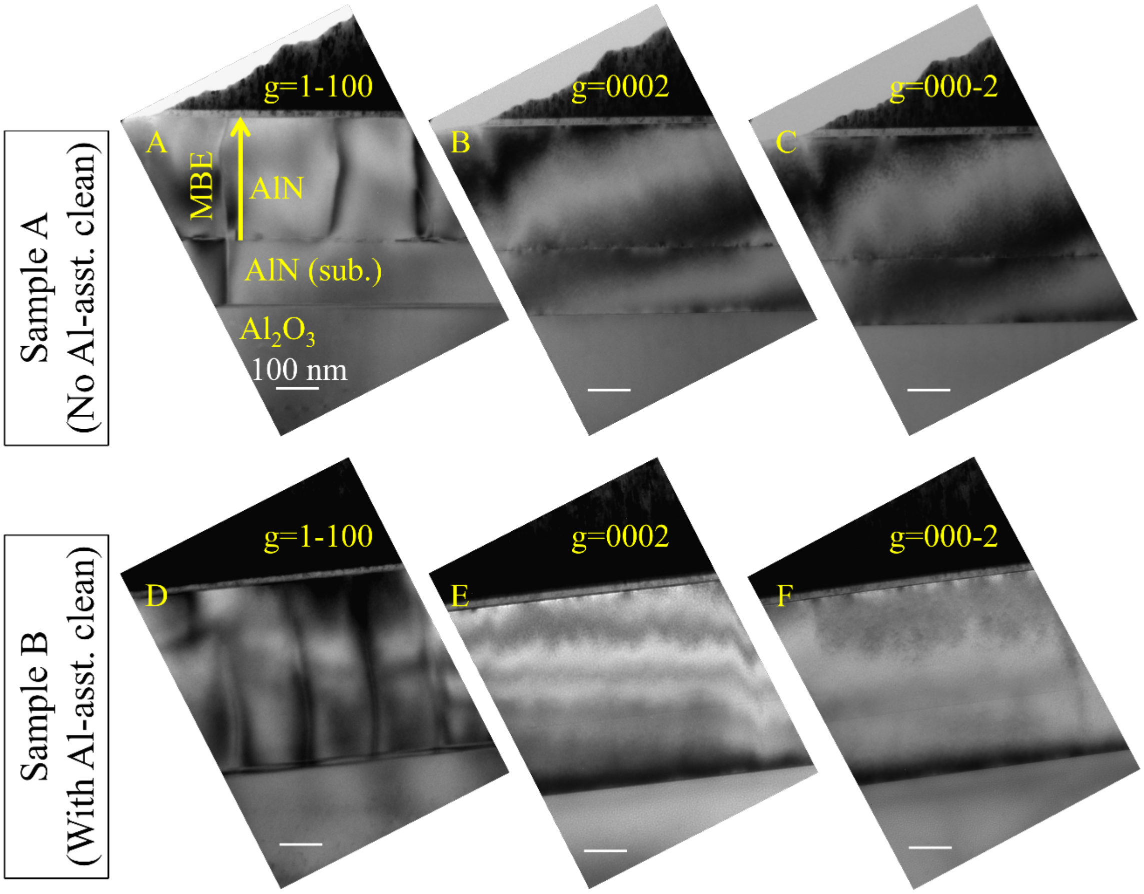


**Fig. S2.**

**Two-beam bright-field cross-sectional TEM images of AlN grown on AlN templates.** (**A** to **C**) Sample A and (**D** to **F**) sample B near the <11-20> zone axis with g=1-100 (**A** and **D**), g=0002 (**B** and **E**) and g=000-2 (**C** and **F**).
